# Supplementary material for: Derandomized knockoffs: leveraging e-values for false discovery rate control
Source: arXiv:2205.15461 source file (2023-08-31)
Supplement: Supplementary file 1 [file supplement.tex]

\documentclass{statsoc}

\usepackage[a4paper,top=1.25in, bottom=1.25in, left=1in, right=1in]{geometry}

\usepackage{graphicx}
\usepackage{amsmath}
\usepackage{amssymb}
\usepackage{graphicx}
\usepackage{natbib}
\usepackage{enumitem}
\usepackage{mathtools}
\usepackage{mathrsfs}
\mathtoolsset{showonlyrefs}
\usepackage{tikz}
\usepackage{anyfontsize}
\usepackage[ruled]{algorithm2e}
\usepackage{xr}
\usepackage{hyperref}
\hypersetup{
    colorlinks,%
    citecolor=blue,%
    filecolor=blue,%
    linkcolor=black,%
    urlcolor=blue
}

%%input macros
\input{macro}
\graphicspath{{./figs/}}

\externaldocument{main}

%% Theorems

%% Project-specific commands
  % Indicator

\renewcommand{\citet}{\cite}

% Meta information
\title[Supplementary Material of ``Conformalized Survival Analysis'']{Supplementary Material of ``Conformalized Survival Analysis''}
\author[Author 1 {\it et al.}]{Emmanuel Cand\`es}
\address{Department of Mathematics and Department of Statistics, Stanford University, CA, USA.}
\email{candes@stanford.edu}

\author{Lihua Lei}
\address{Department of Statistics, Stanford University, Stanford, CA, USA.}
\email{lihualei@stanford.edu}

\author{Zhimei Ren}
\address{Department of Statistics, Stanford University, Stanford, CA, USA.}
\email{zren@stanford.edu}

\begin{document}
\appendix
\numberwithin{equation}{section}
\numberwithin{theorem}{section}
\numberwithin{lemma}{section}

\allowdisplaybreaks
\input{appendixEC}

\bibliographystyle{rss}
\bibliography{cfsurv}
\end{document}
